# Supplementary material for: Multimodal Perception for Goal-oriented Navigation: A Survey
Source: arXiv:2504.15643 source file (2025-04-22)
Supplement: Supplementary file 1 [file 9supplement.tex]

\bibliography{ref}
\bibliographystyle{IEEEtran}
\section{Supplementary Material}
\label{sec:supplementary}
\subsection{Additional Details on the PointNav Novel Methods}
\begin{itemize}
    \item \textbf{ANM} \cite{chaplot2020learning} introduces a modular approach for training policies to explore 3D environments. It uses a Neural SLAM module, a global policy and a local policy. The Neural SLAM module takes in RGB observations and agent pose data to output updated maps and pose estimates using a Mapper and a Pose Estimator. The egocentric map from the Mapper transforms into a geocentric map using the Pose Estimator's pose estimate and aggregates with the previous spatial map for an updated map. The global policy then uses the map and agent pose to sample long-term goals using classicla algorithm called Frontier-based exploration (FBE)\cite{yamauchi1997frontier}, while the local policy maps RGB images to actions and achieving short-term goals. 
    \item \textbf{LSP-Unet}\cite{li2022comparison} employs a hierarchical planning framework that integrates a mapping module to build occupancy and semantic maps from RGB-D and semantic segmentation inputs. A U-Net\cite{ronneberger2015u} architecture is trained to estimate frontier properties (e.g. probability of leading to the goal, exploration cost) using supervised learning on partial semantic maps and goal position data.  These learned properties enable the model-based planner to evaluate subgoals via a Bellman equation, combining frontier exploration with Dijkstra-based local path planning for efficient navigation. The mapping module updates iteratively as the agent moves, ensuring robustness to sensor noise while leveraging semantic priors for decision-making. 
    \item \textbf{VO}\cite{zhao2021surprising} employs a ResNet-18 backbone\cite{he2016deep} to estimate SE(2) transformations between consecutive RGB-D frames, integrating four input modalities (RGB, raw depth, discretized depth for noise robustness, and egocentric top-down projections) to capture spatial relationships. Action-specific VO submodels for \textit{forward motion}, \textit{left turns}, and \textit{right turns} improve accuracy by tailoring predictions to distinct movement patterns, while dropout layers in fully connected layers enhance noise tolerance. The training framework combines regression loss for ground-truth pose estimation with geometric invariance losses that enforce consistency under observation permutations, addressing sensor noise and actuation errors.
    \item \textbf{UPEN}\cite{georgakis2022uncertainty} employs a mapping module based on a UNet encoder-decoder structure\cite{ronneberger2015u} with a ResNet18 backbone for feature extraction. This module takes ground-projected depth observations as input, converting them into a local occupancy grid that classifies regions as occupied, free, or unknown. The UNet is trained via pixel-wise cross-entropy loss to predict complete local occupancy maps, leveraging depth data to infer unobserved areas without relying on RGB inputs. To estimate epistemic uncertainty, the system uses an ensemble of four such UNet models, each initialized with different weights, generating variance-based uncertainty maps by aggregating their predictions. These predictions are integrated into a global map using Bayesian updating\cite{lakshminarayanan2017simple}. The ensemble’s uncertainty estimates guide path selection during exploration and navigation, while the global map dynamically updates as the agent moves, enabling efficient reasoning about partially observed environments.
    \item \textbf{IMN-RPG}\cite{partsey2022mapping} demonstrates that explicit mapping is unnecessary for PointNav by integrating a self-supervised visual odometry (VO) model with reinforcement learning (RL), using VO-predicted egomotion to maintain agent-centric pose estimates (distance/angle to goal) and training an LSTM-based policy on RGB observations, VO poses, and historical states .
    \item \textbf{MoDA (Map Style Transfer for Self-supervised Domain Adaptation)} \cite{lee2022moda} is a self-supervised domain adaptation method for transferring pre-trained embodied agents to new, noisy environments with visual and dynamics corruptions1. It leverages map-based memory, which offers contextual information through its spatial structure of walls and obstacles, to guide the agent in overcoming domain discrepancies. The method employs style transfer networks to generate pseudo-clean maps and encourages inherent regularities on estimated maps. The mapping module uses map-to-map translation networks CycleGAN\cite{zhu2017unpaired} for egocentric and global maps, capturing structural regularities from ground-truth maps and translating them to noisy maps. This module also contains a curriculum learning approach to domain adaptation, using the hierarchical structure of map-based models.
    %better than IMN-RPG
    \item \textbf{MPVO}\cite{paul2024mpvo} enhances point-goal navigation by improving visual odometry (VO) using motion priors and the model architecture is beased on IMN-RPG\cite{partsey2022mapping}. MPVO employs a training-free geometric VO module using action priors to estimate a coarse relative pose. This coarse pose then acts as a motion prior for a deep-learned VO model, which refines the pose for the navigation policy. The approach improves sample efficiency during training and boosts accuracy and robustness in point-goal navigation tasks, outperforming state-of-the-art VO methods.

    \item \textbf{VO}\cite{zhao2021surprising} employs a ResNet-18 backbone\cite{he2016deep} to estimate SE(2) transformations between consecutive RGB-D frames, integrating four input modalities (RGB, raw depth, discretized depth for noise robustness, and egocentric top-down projections) to capture spatial relationships. Action-specific VO submodels for \textit{forward motion}, \textit{left turns}, and \textit{right turns} improve accuracy by tailoring predictions to distinct movement patterns, while dropout layers in fully connected layers enhance noise tolerance. The training framework combines regression loss for ground-truth pose estimation with geometric invariance losses that enforce consistency under observation permutations, addressing sensor noise and actuation errors.
        %better than IMN-RPG
    \item \textbf{MPVO}\cite{paul2024mpvo} enhances point-goal navigation by improving visual odometry (VO) using motion priors and the model architecture is beased on IMN-RPG\cite{partsey2022mapping}. MPVO employs a training-free geometric VO module using action priors to estimate a coarse relative pose. This coarse pose then acts as a motion prior for a deep-learned VO model, which refines the pose for the navigation policy. The approach improves sample efficiency during training and boosts accuracy and robustness in point-goal navigation tasks, outperforming state-of-the-art VO methods.
    \item \textbf{IMN-RPG}\cite{partsey2022mapping} demonstrates that explicit mapping is unnecessary for PointNav by integrating a self-supervised visual odometry (VO) model with reinforcement learning (RL), using VO-predicted egomotion to maintain agent-centric pose estimates (distance/angle to goal) and training an LSTM-based policy on RGB observations, VO poses, and historical states .
        %SplitNet's main contribution lies in Sim2Sim and Task2Task transfer rather than a direct enhancement of PointNav performance via auxiliary tasks
    \item \textbf{SplitNet} \cite{gordon2019splitnet} decouples visual perception from policy learning through two specialized components. The visual encoder combines multi-task geometric objectives - explicit depth mapping, surface normal orientation analysis, egomotion calculation, and future frame feature prediction. A gradient-isolated bidirectional LSTM policy network then translates these geometric priors into navigation actions through temporal state tracking. The design enables:
    \begin{itemize}
        \item Sim2Sim transfer via encoder fine-tuning with target-domain geometric tasks
        \item Task2Task adaptation through policy network retraining while maintaining original visual representations through gradient blocking.
    \end{itemize}
        
    \item \textbf{Attention Fusion} \cite{ye2021auxiliary} integrates three self-supervised objectives: 
    \begin{itemize}
        \item action-conditional contrastive predictive coding (CPC$|$A)\cite{guo2018neural} for multi-step dynamics modeling.
        \item inverse dynamics\cite{pathak2017curiosity} for action prediction.
        \item Temporal distance estimation for trajectory coherence.
    \end{itemize}
    There is a shared ResNet-18 encoder feeds into parallel GRU belief modules\cite{cho2014learning} with spatial-temporal attention gates dynamically fusing task-specific features. Joint optimization with entropy-regularized attention weights prevents task dominance while enabling synergistic environment reasoning.
        
    \item \textbf{Efficient learning} \cite{desai2021auxiliary} introduces three synergistic auxiliary tasks - depth prediction (discretized spatial geometry reconstruction), inverse dynamics (action transition modeling) and path length regression (geodesic progress estimation). These connect to a central GRU policy network that spatially separates geometric processing (CNN feature maps) from temporal state evolution (GRU hidden states). Multi-task optimization accelerates policy convergence by decoupling visual feature acquisition from sparse reward signals.
    
    \item \textbf{DD-PPO}\cite{wijmans2019dd} redefined scalability in embodied RL, enabling unprecedented performance in PointNav that solve the limitation of PPO\cite{schulman2017proximal} in scaling as the high dimentional inputs(e.g., RGB-D frames) and slow convergence. Its decentralized design and transferable policies serve as a backbone for next-gen navigation systems, though challenges in generalization and sensor independence persist. Future work may integrate language models or address sim2real gaps through adaptive pretraining.
    \item \textbf{DD-PPO Depth}\cite{weihs2020allenact} extends the original DD-PPO by integrating depth-specific enhancements for embodied navigation. This modular framework introduces depth-based auxiliary tasks (e.g., surface normals prediction) and multi-stage curriculum learning, enabling agents to achieve 97.3\% success on PointNav with 10x less data (250M frames vs. DD-PPO's 2.5B) through improved regularization and structured training pipelines.
    \item \textbf{Ego-Localization}\cite{datta2021integrating} incorporates a pre-trained CNN-based visual odometry module to estimate egomotion, enabling agents to navigate without perfect localization and with noisy actions and a recurrent neural network (LSTM) policy network that predicts actions based on visual input, previous actions, and goal coordinates. The policy network is trained using DD-PPO\cite{wijmans2019dd}, with a reward function that encourages success, efficient exploration, and reaching the target.
    \item \textbf{RobustNav}\cite{chattopadhyay2021robustnav} processes sequential observations (RGB-D inputs, GPS, and compass data) through a Gated Recurrent Unit (GRU) to model temporal dependencies and maintain a hidden state representing the agent's internal navigation context. This policy maps sensory inputs to action probabilities (e.g., move forward, turn left/right) using a multi-layer perceptron (MLP) head, enabling iterative goal-directed navigation. The study evaluated robustness by exposing the GRU policy to visual corruptions (e.g., noise, blur) and dynamics perturbations (e.g., actuation noise), revealing performance degradation under such conditions.
    \item \textbf{iSEE} \cite{dwivedi2022navigation} employs a GRU-based policy for PointNav that integrates GPS+compass inputs (providing target distance $R_t$ and orientation $\theta_t$ with visual observations from a ResNet18 or SimpleConv encoder12. The GRU dynamically encodes agent-centric spatial progress, including the distance from the initial spawn location ($R_a$), through a combination of recurrent hidden states and sensor data.
    \item \textbf{ENTL} \cite{kotar2023entl} introduces a method for learning navigation trajectories by training a spatio-temporal transformer model\cite{chen2021decision} to encode sequences of images, actions, and poses. The model predicts future frames, actions, and poses, unifying world modeling, localization, and imitation learning into a single sequence prediction task. The architecture shares a backbone across tasks like future frame prediction, agent localization, and navigation, relying on treating observations and actions as part of a long contiguous sequence. The model is trained using VQ-GAN\cite{esser2021taming} tokens predictions of future states conditioned on current states and actions and it is pre-trained without any explicit reward signal, making it generalizable to multiple tasks and environments.
\end{itemize}

\subsection{Additional Details on the ObjectNav Novel Methods}
\begin{itemize}
    \item \textbf{VTNet}\cite{du2021vtnet} utilizes spatial-aware descriptors, including a spatial-enhanced local descriptor DETR\cite{carion2020end} that leverages detected objects and their spatial relationships, and a positional global descriptor that incorporates positional embeddings of image regions and it is similar to SAVN\cite{wortsman2019learning}, which adopts ResNet18\cite{he2016deep} pretrained on ImageNet\cite{deng2009imagenet}. A pre-training scheme is used to associate visual representations with directional navigation signals, which facilitates navigation policy learning using an LSTM-based navigation policy network and the A3C architecture. Therefore, VTNet effectively navigation by encoding relationships among objects and establishing strong correlations with navigation signals.

    \item \textbf{DRL}\cite{kulhanek2021visual,kulhanek2019vision} explores deep reinforcement learning for visual navigation and \cite{kulhanek2021visual} emphasizes the real-world application and leveraging a sophisticated neural network architecture, which comprises convolutional layers for image processing, an LSTM layer\cite{schmidhuber1997long} for handling sequential data, and multiple heads for auxiliary tasks such as image reconstruction and reward prediction, is trained using the Parallel Advantage ActorCritic (PAAC) algorithm\cite{clemente2017efficient} with off-policy critic updates. This setup enables the agent to make decisions based on visual input. The training process begins in a simulated environment with domain randomization to enhance adaptability then followed by fine-tuning with real-world data to ensure generalization. 
    
    \item \textbf{DITA(Depth-Inference Termination Agent)}\cite{song2023learning} incorporates a Judge Model and a supervised classification model in order to implicitly infer object-wise depth and decide termination jointly with reinforcement learning. The Judge Model is trained alongside the DRL agent using the DRL reward signal to assess the appropriate termination time. The DRL branch uses MJOLNIR-o\cite{pal2021learning} as backbone model, the branch involves observation embedding, Node Feature Matrix construction, Context Matrix construction, joint embedding\cite{pennington2014glove} with an LSTM cell. Leveraging the GNN processes object relations from the Visual Genome(VG) dataset\cite{krishna2017visual} to create node embeddings that capture semantic relationships. Those embeddings is along with a Context Matrix that provides current object detection states then passing into LSTM cell, which manages the temporal dynamics of the agent's navigation by remembering past actions and observations. The A3C algorithm utilizes the LSTM's output to learn the control action distribution.
    
    \item \textbf{RIM(Recursive Implicit Map)}\cite{10341827} employs a spatial grid of latent vectors that are recursively updated as the agent explores the environment, capturing both geometry and semantics without explicit map construction. The multi-layer transformer\cite{waswani2017attention} is central to processing spatial relationships and sequence data, enabling effective RIM updates. Furthermore, auxiliary tasks such as visual feature prediction, explicit map reconstruction, and semantic prediction enhance the model's environmental understanding and navigation performance.
    
    \item \textbf{OMT(Object Memory Transformer)}\cite{fukushima2022object} integrates a long-term memory system (OSM) with a Transformer-based\cite{waswani2017attention} inference mechanism. The Object-Scene Memory (OSM), which stores long-term observations of scenes and objects, enabling the agent to remember past interactions. The Transformer acts as the inference domain, processing these memory by leveraging attention mechanisms to focus on relevant parts of the stored data and effectively handling long-term dependencies that are crucial for navigation. By incorporating temporal encoding\cite{mikolov2013efficient}, the Transformer maintains an understanding of the sequence of events, enhancing its ability to make informed decisions.

    \item \textbf{Habitat-web}\cite{ramrakhya2022habitat} leverages a large-scale dataset of human demonstrations collected via a web-based teleoperation infrastructure. The study compares imitation learning (IL) agents trained on this dataset with reinforcement learning (RL) agents, finding that IL outperforms RL in both ObjectGoal Navigation and Pick\&Place tasks. Specifically, IL agents demonstrated the ability to learn and mimic efficient object-search behaviors observed in human demonstrations such as peeking into rooms and checking corners, which are not typically exhibited by RL agents.The agent also utilizes a GPS+Compass sensor for location and orientation. In addition to RGBD and GPS+Compass data, semantic segmentation (SemSeg) and a 'Semantic Goal Exists' (SGE) scalar are used as semantic features. These features are computed using a pretrained and frozen RedNet\cite{jiang2018rednet} pretrained on SUN RGB-D\cite{song2015sun} and finetuned on 100k randomly sampled views in the Habitat simulator. All input features are then concatenated and fed into GRU\cite{cho2014learning} at every timestep. The results suggest that human demonstrations provide valuable information for learning effective exploration strategies and that simply collecting more demonstrations is likely to further advance the state of the art in embodied AI.
    
    \item \textbf{HiNL(History-inspired Navigation Learning)}\cite{Du2023ObjectGoalVN} does effectiely navigation through explicitly modeling relationships among historical navigation states. HiNL addresses the issue of high relevance among navigation states in existing methods, which leads to inefficient exploration. The framework consists of two key components: History-aware State Estimation (HaSE), which estimates states more responsive to current visual observations by mitigating the influence of dominant historical states, and History-based State Regularization (HbSR), which constrains correlations among navigation states during training to promote more effective state updates. 

    \item \textbf{OVRL}\cite{yadav2023ovrl} integrates Vision Transformers (ViTs)\cite{alexey2020image}, compression layers, and Long Short-Term Memory (LSTM) networks, The ViTs process input RGB images by dividing them into patches and encoding them but it will preserve critical spatial information for navigation. This compressed representation is concatenated with a goal embedding. The combined features are then fed into an LSTM, which captures temporal dynamics and past states to output action probabilities for action decition. Key findings include the necessity of compression layers to retain spatial information when using ViTs for navigation, and the demonstration of positive scaling laws through visual pretraining using Masked Autoencoders (MAE)\cite{he2022masked} on in-domain data.  Furthermore, the study addresses limitations in existing reward functions\cite{al2022zero} by proposing a correction that mitigates reward hacking\cite{ng1999policy}.
    
    \item \textbf{PIRLNav}\cite{ramrakhya2023pirlnav} employs a two-stage learning architecture to enhance Object Goal Navigation (OBJECTNAV) by integrating behavior cloning (BC) pretraining on human demonstrations with reinforcement learning (RL) finetuning. The BC pretraining phase utilizes a policy, denoted as $\pi_\theta^{BC}(a_t|o_t)$, which maps observations $o_t$ to action distributions $a_t$ based on trajectories of state, observation, and action tuples. The optimal parameters are determined by minimizing the negative log-likelihood of the action distribution across all demonstrations, with an inflection weighting technique applied to emphasize timesteps where actions change. The architecture features a simple CNN+RNN model from\cite{yadav2023offline}, specifically using a ResNet50\cite{he2016deep} for RGB input encoding and a 2-layer GRU for action prediction. Additionally, the study reveals that human demonstrations which is collect by using habitat-web\cite{ramrakhya2022habitat} significantly outperform other sources such as shortest paths or task-agnostic exploration in facilitating effective BC-RL transfer, while also identifying key failure modes related to dataset issues and navigation challenges.
    
    \item \textbf{OVON}\cite{yokoyama2024hm3d} highlights the effectiveness of a transformer-based architecture and empploy frozen SigLIP\cite{zhai2023sigmoid} RGB and text encoders to encode the visual observations and the goal object category. These encoders have been identified as highly effective for ObjectNav by\cite{ehsani2023imitating}. Key finding that DAgger\cite{ross2011reduction} pre-training with frontier exploration trajectories, followed by RL fine-tuning (DAgRL), achieves superior performance compared to other end-to-end methods. However, the modular method VLFM\cite{yokoyama2024vlfm} demonstrates better generalization to unseen object categories, attributed to its use of an open-vocabulary object detector(OWLv2)\cite{minderer2024scaling}. Augmenting DAgRL with an object detector(DAgRL+OD) significantly improves generalization and robustness to noise. The transformer's ability to handle sequential observations is significant in achieving outperforming in HM3D-OVON open-vocabulary setting.
\end{itemize}

\subsubsection{Latent Map Inference Domain model detail}
\begin{itemize}
    \item \textbf{Sem-EXP}\cite{chaplot2020object} implements a modular architecture for object goal navigation centered on a latent semantic map representation. The framework constructs an episodic semantic map that integrates geometric and semantic information through differentiable projections\cite{chaplot2020learning}. Environmental understanding is enhanced through a pretrained Mask R-CNN\cite{he2017mask} for object detection and segmentation, with map refinement performed via a denoising network. A Goal-Oriented Semantic Policy learns to select long-term navigation goals by interpreting the semantic map representation, moving beyond the limitations of myopic end-to-end approaches. The latent map serves as both a memory structure and an active inference domain for navigation decision-making.
    \item \textbf{HISNav}\cite{HISNav} integrates deep learning techniques with hierarchical reinforcement learning to address the challenges of real-time object navigation, particularly in environments with sensor and actuator noise. HISNav is designed around three key subtasks: instance segmentation of target objects, ego-motion estimation and localization through ORB-SLAM2\cite{mur2017orb}, and automatic exploration and path planning. The authors developed a novel dataset named the HISNav dataset that is based on the Habitat simulation environment\cite{savva2019habitat}, which facilitates the pre-training of models before deployment on real robotic platforms. The architecture combines semantic segmentation, simultaneous localization and mapping (SLAM)\cite{durrant2006simultaneous}, and a hierarchical reinforcement learning approach that utilizes two levels of policies for effective navigation.
    \item \textbf{L2M(Learning to Map)}\cite{georgakis2021learning} actively learns to predict semantic maps outside the agent's field of view and uses uncertainty estimates derived from an ensemble of segmentation models\cite{lakshminarayanan2017simple} to guide long-term goal selection, balancing exploration and exploitation. Key components include an active training strategy that selects samples based on information gain, uncertainty quantification to identify areas where the model lacks confidence, and a goal navigation policy designed as a POMDP\cite{kaelbling1998planning}. Overall, L2M demonstrates the importance of active learning and uncertainty quantification in enhancing robotic navigation capabilities.
    \item \textbf{Distance map}\cite{zhu2022navigating} constructs a comprehensive latent map representation comprising a bird's-eye view semantic map\cite{chaplot2020learning} and a predicted distance map. The semantic map captures object locations and spatial relationships, while the distance map estimates geodesic distances to potential target locations. By leveraging learned spatial correlations between objects\cite{wang2018efficient,kunze2014using}, the architecture dynamically updates both maps as the agent explores, enabling informed selection of mid-term navigation goals. The system prioritizes exploration of areas predicted to minimize the distance to target objects, leading to more efficient navigation trajectories\cite{sethian1996fast}.
    \item \textbf{PEANUT(Predicting and Navigating to Unseen Targets)}\cite{Zhai_2023_ICCV} employs a global semantic map as its latent inference domain, which dynamically integrates diverse environmental data for predicting unseen target locations. The architecture utilizes PSPNet\cite{zhao2017pyramid} to generate semantic segmentation masks, which are projected onto a top-down semantic map\cite{chaplot2020learning}. The prediction model leverages global context to forecast target probabilities in unexplored areas, guiding efficient path planning by prioritizing closer, high-probability locations. By avoiding reinforcement learning approaches, PEANUT achieves data efficiency while maintaining computational feasibility and robust navigation performance.
    \item \textbf{PONI (Potential Functions for ObjectGoal Navigation with Interaction-free Learning)} \cite{ramakrishnan2022poni} introduces an innovative mapping approach that constructs a 2D top-down semantic map as its primary inference domain. The mapping module dynamically integrates RGB-D observations and agent pose information to create a comprehensive representation encompassing obstacles, explored regions, and object categories \cite{chaplot2020learning}. The architecture's key innovation lies in its dual potential function network that generates complementary potentials: the first potential guides efficient frontier-based exploration \cite{yamauchi1997frontier}, while the second enables goal-directed navigation through geodesic distance metrics \cite{sethian1996fast}. This dual-potential approach allows the agent to balance between exploration of unknown areas and exploitation of known information about the target object's potential location. The semantic mapping system maintains spatial consistency through geometric projections and updates, enabling robust navigation in complex environments without requiring interaction-based training.
    \item \textbf{RNR-Map(renderable neural radiance map)}\cite{kwon2023renderable} introduces a novel grid-based mapping approach that employs latent codes derived from image observations to encapsulate environmental visual information. The latent codes are embedded into grid cells and can be transformed into a neural radiance field\cite{mildenhall2021nerf} for image rendering, facilitating crucial tasks such as localization and navigation. The architecture implements an efficient encoding mechanism that transforms images into latent codes and maps them into a grid structure based on their 3D positions through inverse projection\cite{hartley2003multiple}. Similar to previous work in neural scene representations\cite{tancik2022block,muller2022instant}, the latent map serves as the primary inference domain, where visual information is processed to identify similar locations through feature matching\cite{lowe2004distinctive}, enabling robust and accurate navigation in complex environments.
    \item \textbf{3D-Aware}\cite{zhang20233d} advances navigation in unknown environments through sophisticated 3D scene understanding. The framework constructs detailed 3D maps using online semantic point fusion\cite{dai2017scannet,zhang2020fusion}, achieving superior precision compared to traditional 2D maps\cite{chaplot2020learning} or scene graphs\cite{zhu2021soon}. The architecture integrates two key components: a corner-guided exploration policy that strategically directs the agent towards scene corners and a category-aware identification policy that ensures reliable target recognition through semantic consistency checks\cite{qi2017pointnet}. These components are optimized using Proximal Policy Optimization (PPO)\cite{schulman2017proximal}, resulting in robust navigation performance. The empirical results demonstrate significant improvements in both exploration efficiency and target identification accuracy.
    \item \textbf{LocCon}\cite{10341959} introduces a "Location Consistency" (LocCon) approach that enables training without expensive labeled 3D mesh data through a two-stage process. In Stage I, the system fine-tunes a semantic segmentation model\cite{chen2017deeplab} using contrastive learning\cite{chen2020simple} on multi-viewpoint images from identical locations, enhancing object recognition capabilities across varying perspectives. Stage II leverages these self-labeled semantic maps to develop a navigation policy that optimally balances exploration and exploitation through potential functions over map frontiers\cite{yamauchi1997frontier}. The architecture emphasizes in-situ finetuning, facilitating adaptation to real-world environments through direct learning from unannotated image data. This self-supervised approach demonstrates robust performance in object goal navigation tasks while significantly reducing the dependency on manually annotated training data, achieving comparable results to fully supervised methods\cite{chaplot2020learning}.
    \item \textbf{StructNav}\cite{chen2023not} presents a training-free approach by integrating classical navigation techniques with semantic reasoning. The framework constructs a structured scene representation through Visual SLAM (V-SLAM)\cite{mur2015orb}, comprising a 2D occupancy map, semantic point cloud, and spatial scene graph. The method enhances frontier-based exploration\cite{yamauchi1997frontier} with semantic scoring using pre-computed prior matrices derived from language models (BERT\cite{devlin2018bert}, CLIP\cite{radford2021learning}). This semantic integration enables the agent to prioritize exploration areas with higher probability of containing the target object, based on learned semantic relationships\cite{mikolov2013distributed}.
        
    \item \textbf{DDN(Demand-driven Navigation)}\cite{wang2024find} implements a novel approach that extracts common-sense knowledge from large language models (LLMs) to address demand-conditioned navigation. The framework learns textual attribute features from LLM-generated descriptions, which are then aligned with visual features through CLIP embeddings\cite{radford2021learning}. The architecture comprises three key components: a textual attribute feature learning module that leverages LLMs for reasoning about object attributes, a textual-visual alignment mechanism utilizing CLIP for grounding semantic knowledge and a policy learning component incorporating a visual grounding model. The method is evaluated on a carefully curated DDN dataset constructed through GPT-3 generation\cite{brown2020language}, manual verification and systematic augmentation. Empirical results demonstrate the effectiveness of this approach in enabling agents to navigate and identify objects that satisfy specific user demands while maintaining robust generalization capabilities.
    \item \textbf{L3mvn}\cite{yu2023l3mvn} integrates large language models to impart common-sense knowledge about objects and layouts~\cite{brown2020language,devlin2018bert}. The architecture comprises three main components: semantic map construction, frontier detection~\cite{yamauchi1997frontier} and frontier selection using two distinct paradigms. In the zero-shot paradigm, a pre-trained language model evaluates descriptive sentences about frontier areas and target objects to guide exploration. The feed-forward paradigm utilizes language model embeddings and a fine-tuned neural network to assess frontier relevance~\cite{radford2021learning}. For local navigation between frontiers, the framework implements efficient path planning through methods such as Fast Marching~\cite{sethian1996fast}. This approach demonstrates the effectiveness of leveraging linguistic knowledge for enhanced navigation performance without requiring extensive task-specific training.
    \item \textbf{SGM(Self-Supervised Generative Map)}\cite{zhang2024imagine} introduces an innovative approach for predicting unobserved environmental regions to facilitate object-goal navigation in novel settings. Drawing inspiration from masked modeling techniques\cite{he2022masked}, the framework employs a multi-scale training strategy where global semantic maps are systematically cropped and partially masked at varying scales and orientations. The model's architecture integrates visual observations with semantic knowledge extracted from large language models (GPT-4\cite{achiam2023gpt}, ChatGLM\cite{du2021glm}) to predict masked regions. The predicted completions guide the agent's exploration by providing probabilistic estimates of target object locations, enabling more efficient long-term goal setting through informed spatial reasoning\cite{chaplot2020learning,ramakrishnan2022poni}.
    \item \textbf{NOMAD}\cite{sridhar2024nomad} introduces a sophisticated diffusion-based policy approach to predict unobserved environmental regions and optimize exploration strategies. Unlike preceding methodologies that employ distinct policies for exploration and goal-directed behaviors\cite{chaplot2020learning,ramakrishnan2022poni}, NOMAD implements a unified model architecture for both tasks. Building on foundational work in denoising diffusion probabilistic models~\cite{song2020score,ho2020denoising,dhariwal2021diffusion}, the framework mathematically approximates the conditional distribution $p(a_t|c_t)$, where $c_t$ represents the observation context derived from ViNT's~\cite{shah2023vint} attention-based encoding mechanisms. The architecture incorporates a novel goal-masking technique that enables conditional inference through binary masking operations, effectively controlling information flow during the decision process~\cite{vaswani2017attention}. The diffusion policy component employs a 1D conditional U-Net structure to capture and model multimodal action distributions that naturally emerge in complex navigation scenarios~\cite{sohl2015deep,song2020score}. Extensive empirical evaluations demonstrate NOMAD's efficacy in learning object placement distributions and spatial relationships, enabling probabilistic reasoning about plausible semantic maps~\cite{lugmayr2022repaint,poole2022dreamfusion} while guiding exploration in previously unseen environments with superior adaptability and generalization capabilities~\cite{ramesh2022hierarchical,karras2022elucidating}.

    \item \textbf{DAR (Diffusion As Reasoning)}\cite{ji2024diffusion} employs diffusion models as a sophisticated inference tool for navigation in unseen environments. Drawing inspiration from recent advances in diffusion modeling~\cite{ramesh2022hierarchical,saharia2022photorealistic}, the system generates plausible semantic maps of unexplored areas conditioned on known environmental features. The architecture integrates two key components: a "global target bias" that guides the generation process toward likely target object locations, and a "local LLM bias" that incorporates common-sense knowledge from large language models about object relationships~\cite{brown2020language}. This dual-bias approach enables semantic reasoning about potential object placements while maintaining consistency with observed environmental structure~\cite{karras2022elucidating}.
    
    \item \textbf{T-Diff} \cite{yu2024trajectory} introduces a novel trajectory diffusion approach for object goal navigation (ObjectNav) that reconceptualizes embodied navigation as a generative modeling challenge. Unlike conventional methods relying on single-step reactive planning, T-Diff employs a denoising diffusion probabilistic model (DDPM) to generate temporally coherent trajectory sequences conditioned on visual observations, target object semantics, and partial map representations. By decomposing navigation into distinct trajectory generation and trajectory following phases, the system achieves superior planning capabilities through hierarchical reasoning. The model, trained via self-supervised learning on automatically collected optimal trajectories, iteratively transforms random noise into coherent trajectory representations through a Transformer-based diffusion process. Experimental results demonstrate enhanced scalability across simulation environments, indicating robust generalization capabilities. This work represents a paradigm shift from traditional reactive navigation approaches by explicitly modeling navigation as a continuous trajectory generation problem within a unified probabilistic framework, aligning with recent advances in diffusion-based generative modeling \cite{ho2020denoising,song2020score}.

    \item \textbf{EmbCLIP}\cite{khandelwal2022simple} presents a simple yet effective approach that leverages frozen CLIP ResNet-50\cite{he2016deep,radford2021learning} embeddings for embodied AI tasks. The architecture processes RGB images and integrates them with goal specifications through a GRU\cite{cho2014learning}, enabling effective action prediction. This streamlined approach outperforms more complex architectures on various navigation-heavy tasks without requiring additional sensory inputs. Through extensive probing experiments, the study demonstrates CLIP embeddings' capability to capture essential semantic and geometric information crucial for navigation.

    \item \textbf{ZSEL(zero-shot experience learning)}\cite{al2022zero} presents a unified approach to semantic visual navigation through modular transfer learning for zero-shot generalization. The architecture comprises several key components: a semantic search policy for image goals trained with a novel reward function that optimizes view alignment\cite{mirowski2016learning} and complemented by task augmentation techniques\cite{tobin2017domain} to enhance generalization capabilities. To enable cross-modal transfer, the framework learns a joint goal embedding space offline that allowing various input modalities (sketches, audio, category names) to align with image goals through embedding alignment\cite{radford2021learning,chen2020simple}. This modular approach facilitates efficient transfer of learned components to novel tasks without task-specific training, achieving robust performance across diverse navigation scenarios\cite{anderson2018vision,batra2020objectnav}.
    \item\textbf{COWs}\cite{gadre2023cows} addresses language-driven zero-shot object navigation by leveraging CLIP embeddings\cite{radford2021learning} to enable navigation to language-specified objects without prior training. The architecture integrates depth-based mapping for environmental understanding\cite{chaplot2020learning}, employing object localization techniques powered by CLIP to identify target objects. The system incorporates both frontier-based exploration strategies\cite{yamauchi1997frontier} and learned policies\cite{schulman2017proximal} to effectively balance exploration and goal-directed navigation. Through extensive evaluation, COWs demonstrates robust generalization capabilities across unseen objects and environments while maintaining computational efficiency through its modular design.
    \item\textbf{ZSON}\cite{majumdar2022zson} demonstrates zero-shot goal navigation capabilities by leveraging CLIP embeddings\cite{radford2021learning} as the primary reasoning component. The framework enables agents to interpret goals specified through various modalities, including images and natural language, via a shared embedding space. Training is conducted on image-goal navigation tasks across diverse, unannotated 3D environments, utilizing a ResNet-50\cite{he2016deep} encoder for observation processing coupled with an LSTM-based policy network for action decision-making. The architecture's effectiveness stems from CLIP embeddings' ability to establish a unified semantic space for goals, facilitating generalization to novel object categories without requiring additional training. This approach aligns with recent advances in vision-language navigation\cite{anderson2018vision,shridhar2020alfred} while maintaining computational efficiency through its streamlined design.
    \item\textbf{VLFM}\cite{yokoyama2024vlfm} integrates frontier-based exploration\cite{yamauchi1997frontier} with vision-language embeddings to enable efficient semantic navigation in unfamiliar environments. The architecture constructs an occupancy map from depth observations to identify frontiers between explored and unexplored areas\cite{chaplot2020learning}. A value map is then generated using BLIP-2\cite{li2023blip} by computing cosine similarity scores between current RGB observations and a text prompt describing the target object. These semantic similarity scores guide frontier selection for exploration. The framework also incorporates state-of-the-art object detection models including YOLOv7\cite{wang2023yolov7} and Grounding-DINO\cite{liu2024grounding}, along with Mobile-SAM\cite{zhang2023faster} for instance segmentation, enabling robust target object localization directly from RGB inputs. This multi-modal approach demonstrates strong zero-shot generalization capabilities while maintaining computational efficiency through its modular design.

    \item\textbf{ESC}\cite{zhou2023esc} leverages pre-trained models to bridge the gap between scene understanding and navigation decisions. The architecture comprises three integral components: (1) open-world scene understanding using the Grounded Language-Image Pre-training (GLIP)\cite{li2022grounded} model for detecting objects and rooms through prompt-based grounding, (2) commonsense reasoning utilizing Large Language Models (LLMs)\cite{brown2020language} to infer spatial relationships between objects and rooms and (3) guided exploration employing Probabilistic Soft Logic (PSL)\cite{bach2017hinge} to convert these inferences into actionable navigation strategies. Building upon recent advances in vision-language models\cite{li2022grounded,radford2021learning} and commonsense reasoning, the architecture emphasizes linguistic inference by integrating textual prompts and probabilistic outputs from LLMs, enabling the agent to reason about the most likely locations of goal objects without prior training on specific environments or objects.
    \item\textbf{OpenFMNav}\cite{kuang2024openfmnav} leverages multiple vision-language models in a modular framework for zero-shot object navigation. The architecture comprises several key components: ProposeLLM for parsing natural language instructions into object candidates, DiscoverVLM for dynamic object detection drawing from approaches in open-vocabulary scene understanding\cite{du2021glm,devlin2018bert}, PerceptVLM for real-time object detection and instance segmentation\cite{zhang2023faster,he2017mask}, and a Versatile Semantic Score Map (VSSM) that maintains a 2D semantic representation integrating multi-modal observations\cite{chaplot2020learning}. ReasonLLM employs common sense reasoning\cite{brown2020language,chowdhery2023palm} on the semantic map to guide exploration strategies, demonstrating robust generalization across novel environments and object categories.
    \item\textbf{Voronav}\cite{wu2024voronav} employs a Reduced Voronoi Graph (RVG)\cite{aurenhammer1991voronoi} to identify key navigation points, enabling agents to explore and locate objects in unfamiliar environments without prior training. The architecture leverages large language models (LLMs)\cite{brown2020language,chowdhery2023palm} to analyze text descriptions of paths and egocentric views, facilitating decision-making through commonsense reasoning\cite{thoppilan2022lamda}. This hierarchical approach integrates a global module for high-level planning with a local policy for action execution\cite{kaelbling1998planning}, demonstrating robust performance in zero-shot navigation tasks while maintaining computational efficiency.
    \item\textbf{SG}\cite{yin2024sgnav} constructs an online 3D scene graph for embodied navigation, representing objects, groups and rooms as interconnected nodes through relational edges\cite{johnson2015image}. The architecture employs hierarchical chain-of-thought prompting with large language models (LLMs) to enable context-aware decision-making. A key innovation is the integration of a re-perception mechanism that leverages visual grounding and semantic reasoning to correct potential goal object misidentifications, enhancing the robustness of zero-shot navigation in novel environments.

    \item \textbf{PixNav}\cite{cai2024bridging} introduces a novel approach to visual navigation by utilizing a transformer-based architecture that processes pixel-level goals from RGB observations. The framework employs dual ResNet18 encoders\cite{he2016deep} for processing both goal pixels and sequential observations, it integrated through a transformer decoder\cite{waswani2017attention} for temporal reasoning. The architecture incorporates three key components: a pixel tracking mechanism inspired by recent advances in visual attention\cite{dosovitskiy2020image}, a temporal distance prediction module following methodologies from visual navigation\cite{anderson2018vision}, and a foundation model interface utilizing Llama-Adapter\cite{zhang2023llama} and GPT-4\cite{achiam2023gpt} for high-level planning through structured prompting\cite{wei2022chain}. This multi-modal approach demonstrates robust performance in pixel-goal navigation while maintaining interpretability through its modular design.
\end{itemize}

\subsection{Additional Details on ImageNav Novel Method}
\begin{itemize}
    \item \textbf{EmerNav}~\cite{bono2023end} incorporates a correspondence network to estimate matching features between views~\cite{weinzaepfel2022croco}, enabling direct navigation without explicit map construction or planning mechanisms.
    
    \item \textbf{NUENav}~\cite{wang2024enhancing} leverages Neural Radiance Fields (NeRF)~\cite{mildenhall2021nerf} as a cognitive structure, NUENav estimates uncertainty to enhance exploratory behavior, enabling efficient environmental cognition and target exploitation. The framework operates in an end-to-end manner, generating cognitive representations while extracting both uncertainty and spatial features from NeRF~\cite{gao2022nerf}. 

    \item \textbf{MANav}~\cite{mezghan2022memory} comprises three principal components designed to enhance navigational performance. Firstly, a data augmentation module improves generalization capabilities through the implementation of random cropping and color jittering techniques, effectively enhancing visual diversity in training data. Secondly, the navigation policy module encodes observations through a shared convolutional neural network (ResNet18), where these representations are systematically concatenated to form a comprehensive joint embedding that informs action selection via Long Short-Term Memory (LSTM) processing pathways. Thirdly, the architecture implements a sophisticated memory module comprising: (i) a self-supervised state-embedding network that learns representations based on temporal proximity principles~\cite{oord2018representation}, (ii) an episodic memory mechanism that maintains a compact representation of previously visited states~\cite{pritzel2017neural,wayne2018unsupervised}, and (iii) an attention-based mechanism for effectively leveraging the stored memory to guide navigation decisions.
    
    \item \textbf{memoNav}~\cite{li2024memonav} integrates three distinct memory representations: short-term memory (STM) for processing transient scene features, long-term memory (LTM) for maintaining persistent environmental representations~\cite{fukuda2009human}, and working memory (WM) that dynamically combines goal-relevant information from both sources. The framework incorporates a selective forgetting mechanism to optimize memory utilization, while employing graph attention networks~\cite{vaswani2017attention} to encode spatial-temporal relationships between observations. This hierarchical memory structure enables efficient information processing through selective retention of goal-relevant features, while the attention-based integration mechanism facilitates adaptive decision-making~\cite{kwon2021visual}.

    \item \textbf{Mod-IIN}~\cite{krantz2023navigating} decomposes navigation into four zero-fine-tuning components: (1) an Exploration Module using frontier-based exploration~\cite{yamauchi1997frontier} to build a 2D occupancy map from depth and pose data, enabling efficient environment coverage; (2) a Goal Instance Re-Identification Module leveraging SuperPoint~\cite{detone2018superpoint} to extract keypoints from images and SuperGlue~\cite{sarlin2020superglue} to compute correspondences, detecting objects by thresholding confidence scores; (3) a Goal Localization Module that segments the goal instance with Detic~\cite{zhou2022detecting}, projects matched keypoints within this mask into world coordinates~\cite{hartley2003multiple}, and creates a navigation target; and (4) a Local Navigation Module implementing fast marching method-based path planning~\cite{sethian1996fast}. Extensive empirical evaluation demonstrates that this modular architecture significantly outperforms end-to-end approaches~\cite{wijmans2019dd} in both success rate and efficiency metrics. The system's effectiveness validates the hypothesis that decomposing complex navigation tasks into specialized modules with well-defined interfaces can yield superior performance while eliminating the need for extensive task-specific training data~\cite{zhu2017target}.
    
    \item \textbf{MIGN}~\cite{wu2022image} consists of  an automatic mapping module that utilizing Neural-SLAM\cite{chaplot2020learning} or Gmapping~\cite{grisetti2007improved}, a long-term goal prediction module employing reinforcement learning~\cite{schulman2017proximal}, a reactive motion planning module implementing Fast Marching Method~\cite{sethian1996fast} or CrowdMove~\cite{fan2018crowdmove} for collision-free navigation and last module for navigation ending prediction module.
    
    \item \textbf{SLING}~\cite{wasserman2023last} presents a modular architecture for visual navigation that integrates three specialized components for robust goal-directed navigation. The Perception Module leverages neural keypoint descriptors~\cite{detone2018superpoint} to establish correspondences between current observations and goal images, while incorporating recent advances in feature matching~\cite{sarlin2020superglue}. The Decision-Making Module employs perspective-n-point (PnP) algorithms~\cite{lepetit2009epnp} enhanced with an adaptive exploration-exploitation mechanism for pose estimation and strategic planning. The Action Module translates high-level navigational decisions into low-level control commands through a learned policy network~\cite{schulman2017proximal}. 

    \item \textbf{LiteVLoc}~\cite{jiao2024litevloc} advances navigation through a hierarchical localization framework that employs a lightweight topo-metric mapping approach. The architecture implements a coarse-to-fine visual localization strategy through three sequential processing modules. The Global Localization module leverages the pre-trained CosPlace model~\cite{berton2022rethinking} for visual place recognition and initializes camera pose estimation using topological constraints~\cite{wang2020atloc}. The Local Localization module refines pose estimates by exploiting covisibility cues from the Covisibility Graph (CvG)~\cite{rublee2011orb}, establishing 2D-3D correspondences that are processed through a PnP solver~\cite{lepetit2009epnp} with RANSAC-based optimization~\cite{fischler1981random}. The Pose SLAM module~\cite{ila2009information} fuses low-rate visual localization results with high-rate sensor odometry~\cite{cadena2016past} to achieve robust real-time pose estimation. This innovative framework significantly reduces computational and storage requirements compared to traditional methods reliant on dense 3D reconstructions~\cite{sarlin2019coarse}, while enhancing adaptability to dynamic environments through its hierarchical design~\cite{sattler2018benchmarking}. Extensive experimental validation across both simulated environments and real-world scenarios demonstrates the system's superior precision and efficiency in large-scale applications, representing a significant advancement in visual localization methodologies for goal-directed navigation tasks.

    \item \textbf{FeudalNav}~\cite{johnson2024feudal} presents a hierarchical approach inspired by feudal learning, avoiding traditional reliance on odometry and metric maps. The architecture comprises three levels: a high-level manager creating a self-supervised Memory Proxy Map (MPM)~\cite{pang2022unsupervised}, a mid-level manager utilizing a Waypoint Network (WayNet) trained on human teleoperation data and a low-level worker executing actions based on waypoints~\cite{sarlin2020superglue}. The key innovations include the MPM for preserving approximate distances between observed images and the WayNet for imitating human navigation strategies.
    
    \item \textbf{TSGM}~\cite{kim2023topological} implements a dual-memory system comprising a topological graph for spatial representation~\cite{savinov2018semi} and semantic features for visual recognition~\cite{he2016deep}. The architecture constructs a sparse topological map during exploration, where nodes represent distinct locations with associated visual observations and edges indicate navigable connections between locations~\cite{chen2019behavioral}. Concurrently, a semantic memory module extracts and stores visual features from observations using a deep convolutional neural network, creating embeddings that enable similarity matching between current observations and the goal image~\cite{gordo2017end}. The reasoning framework employs a hierarchical decision-making process where high-level planning occurs on the topological graph to identify potential paths to the goal~\cite{wortsman2019learning}, while local navigation policies handle obstacle avoidance and path execution. 

    \item \textbf{Mod-IIN}~\cite{krantz2023navigating} decomposes navigation into four zero-fine-tuning components: (1) an Exploration Module using frontier-based exploration~\cite{yamauchi1997frontier} to build a 2D occupancy map from depth and pose data, enabling efficient environment coverage; (2) a Goal Instance Re-Identification Module leveraging SuperPoint~\cite{detone2018superpoint} to extract keypoints from images and SuperGlue~\cite{sarlin2020superglue} to compute correspondences, detecting objects by thresholding confidence scores; (3) a Goal Localization Module that segments the goal instance with Detic~\cite{zhou2022detecting}, projects matched keypoints within this mask into world coordinates~\cite{hartley2003multiple}, and creates a navigation target; and (4) a Local Navigation Module implementing fast marching method-based path planning~\cite{sethian1996fast}. Extensive empirical evaluation demonstrates that this modular architecture significantly outperforms end-to-end approaches~\cite{wijmans2019dd} in both success rate and efficiency metrics. The system's effectiveness validates the hypothesis that decomposing complex navigation tasks into specialized modules with well-defined interfaces can yield superior performance while eliminating the need for extensive task-specific training data~\cite{zhu2017target}.
    
    \item \textbf{MIGN}~\cite{wu2022image} consists of  an automatic mapping module that utilizing Neural-SLAM\cite{chaplot2020learning} or Gmapping~\cite{grisetti2007improved}, a long-term goal prediction module employing reinforcement learning~\cite{schulman2017proximal}, a reactive motion planning module implementing Fast Marching Method~\cite{sethian1996fast} or CrowdMove~\cite{fan2018crowdmove} for collision-free navigation and last module for navigation ending prediction module.
    
    \item \textbf{SLING}~\cite{wasserman2023last} presents a modular architecture for visual navigation that integrates three specialized components for robust goal-directed navigation. The Perception Module leverages neural keypoint descriptors~\cite{detone2018superpoint} to establish correspondences between current observations and goal images, while incorporating recent advances in feature matching~\cite{sarlin2020superglue}. The Decision-Making Module employs perspective-n-point (PnP) algorithms~\cite{lepetit2009epnp} enhanced with an adaptive exploration-exploitation mechanism for pose estimation and strategic planning. The Action Module translates high-level navigational decisions into low-level control commands through a learned policy network~\cite{schulman2017proximal}. 

    \item \textbf{FGPrompt}~\cite{sun2023fgprompt} introduces an innovative fine-grained prompting approach for visual navigation that leverages dual fusion mechanisms to enhance goal-directed reasoning. The framework implements two complementary components: Early Fusion (FGPrompt-EF), which performs pixel-level concatenation of goal and observation images following techniques from visual attention~\cite{mezghan2022memory}, and Mid Fusion (FGPrompt-MF), which employs Feature-wise Linear Modulation (FiLM)~\cite{perez2018film} to dynamically adjust observation encoder activations based on goal image features.
    
    \item \textbf{SimView}~\cite{sakaguchi2024object} integrates three core components: a Vector Registration Module that records feature vectors of observed objects during environment exploration; a Self-Supervised Fine-Tuning Module that employs semantic instance multi-view contrastive learning~\cite{chen2021exploring} to increase similarity between different views of the same object and an Instance Identification Module that calculates cosine similarity between query vectors and registered feature vectors to locate target objects. Experimental validation demonstrated that models trained through unimodal contrastive learning between images significantly outperform multimodal approaches like CLIP~\cite{radford2021learning} for instance-level identification tasks. The researchers further established that fine-tuning pre-trained models with multi-view images collected during robot exploration substantially enhances the system's ability to recognize objects from different viewpoints, as evidenced by improved mean average precision (mAP) scores across multiple test environments. 
    
    \item \textbf{FGPrompt}~\cite{sun2023fgprompt} introduces an innovative fine-grained prompting approach for visual navigation that leverages dual fusion mechanisms to enhance goal-directed reasoning. The framework implements two complementary components: Early Fusion (FGPrompt-EF), which performs pixel-level concatenation of goal and observation images following techniques from visual attention~\cite{mezghan2022memory}, and Mid Fusion (FGPrompt-MF), which employs Feature-wise Linear Modulation (FiLM)~\cite{perez2018film} to dynamically adjust observation encoder activations based on goal image features.
    
    \item \textbf{SimView}~\cite{sakaguchi2024object} integrates three core components: a Vector Registration Module that records feature vectors of observed objects during environment exploration; a Self-Supervised Fine-Tuning Module that employs semantic instance multi-view contrastive learning~\cite{chen2021exploring} to increase similarity between different views of the same object and an Instance Identification Module that calculates cosine similarity between query vectors and registered feature vectors to locate target objects. Experimental validation demonstrated that models trained through unimodal contrastive learning between images significantly outperform multimodal approaches like CLIP~\cite{radford2021learning} for instance-level identification tasks. The researchers further established that fine-tuning pre-trained models with multi-view images collected during robot exploration substantially enhances the system's ability to recognize objects from different viewpoints, as evidenced by improved mean average precision (mAP) scores across multiple test environments. 
\end{itemize}

\subsection{Additional Details on AudioGoalNav Novel Method}
\begin{itemize}
    \item \textbf{VAR} presents a three-component architecture for audio-visual embodied navigation that integrates visual perception mapping, sound localization, and dynamic path planning. The system constructs environment representations through either a key-value based spatial memory during exploration or a 2D occupancy grid for non-exploration settings. It processes stereo audio through Short-Time Fourier Transform (STFT) to generate spectrograms, which are analyzed by a five-layer convolutional network to estimate relative sound source positions. A dynamic path planner then applies Dijkstra's algorithm to compute optimal trajectories based on the constructed spatial graph and audio-derived goal estimates.
    
    \item \textbf{AV-WaN}~\cite{chen2020learning} contributes a learned waypoint prediction framework that constructs spatial audio intensity maps~\cite{gao2020visualechoes} alongside geometric representations, employing neural encoders and a GRU-based temporal integrator~\cite{cho2014learning} to predict intermediate navigation goals. The framework utilizes a hierarchical reinforcement learning approach with two key novel elements: end-to-end learned waypoints within the navigation policy and a structured acoustic memory that provides spatially grounded audio observations~\cite{henriques2018mapnet}. Unlike heuristic-based subgoal approaches~\cite{stein2018learning,bansal2020combining}, AV-WaN adaptively generates waypoints based on environmental complexity and acoustic cues, capitalizing on the synergy of audio and visual data for revealing the geometry of unmapped spaces. Implementation with a modular architecture enables efficient path planning through Dijkstra's algorithm~\cite{schulman2017proximal}, while maintaining robust performance in acoustically complex scenarios. 
    
    \item \textbf{ORAN}~\cite{chen2023omnidirectional} introduces two complementary innovations: Confidence-Aware Cross-task Policy Distillation (CCPD) and Omnidirectional Information Gathering (OIG). CCPD transfers knowledge from PointGoal navigation policies via an entropy-based reweighting mechanism that selectively distills knowledge from confident navigational steps. OIG provides 360-degree environmental awareness by integrating observations from multiple directions (0°, 90°, 180°, 270°). Formulated as a POMDP~\cite{kaelbling1998planning}, the system constructs geometric-acoustic maps with a GRU-based waypoint predictor~\cite{chen2020learning}.

    \item \textbf{CATCH}~\cite{younes2023catch} advances audio-visual navigation by extending static sound localization to dynamic scenarios with moving sound sources in complex, unmapped environments. The framework introduces a novel spatial fusion architecture that integrates depth-constructed geometric maps~\cite{gupta2017cognitive} with binaural audio inputs through specialized encoders that effectively learn cross-modal spatial correlations. Temporal reasoning for sound source tracking is facilitated by a GRU memory component, while a reduced 3×3 action parametrization selects waypoints executed via Dijkstra's algorithm. The authors demonstrate enhanced robustness through comprehensive acoustic complexity scenarios, incorporating distractor sounds, second sounds, and spectrogram augmentations~\cite{park2019specaugment}.
    
    \item \textbf{SDM}~\cite{kondoh2023multi} addresses the challenge of navigating to multiple concurrent sound sources by introducing a novel direction-based representation. The framework enhances audio-visual navigation through a Sound Direction Map that dynamically localizes multiple sound sources in a learning-based manner while utilizing temporal memory. The authors systematically approach the multi-goal audio-visual navigation task by encoding spatial distributions where node values are represented as reciprocals of geodesic distances to sound sources, facilitating more accurate path planning. SDM is integrated with baseline methods such as AV-Nav~\cite{chen2020soundspaces} and SAVi~\cite{chen2021semantic} as a specialized neural network component trained with gradient flows from policy networks and mean squared error calculations. Implementation with Dropout during training enhances robustness by preventing overreliance on previous predictions. Experimental results in SoundSpaces 2.0~\cite{chen2022soundspaces} demonstrate that SDM significantly outperforms conventional approaches across various acoustic conditions, particularly when navigating in scenarios with loud versus quiet sounds, long versus short sounds, and same versus different sound types. 
    
    \item \textbf{SAAVN}~\cite{yu2022sound} formulates audio-visual navigation as a zero-sum two-player game between a navigator and sound attacker to address robustness in complex acoustic environments. The framework implements a novel joint training mechanism utilizing a centralized critic with decentralized actors~\cite{wang2020dop} to ensure stable adversarial learning. The attacker operates within a bounded projection space~\cite{parisotto2020stabilizing}, manipulating positional, volumetric, and categorical sound properties to create acoustically complex scenarios, while the navigator learns resilient policies through competitive optimization. The approach demonstrates considerable robustness when transferred to environments with random intervenors, showcasing enhanced generalization capabilities in naturalistic settings~\cite{schulman2017proximal}. Theoretical analysis confirms the soundness of the approach through proof of attacker observation space boundedness, ensuring productive adversarial training that improves navigation performance rather than degenerating into intractable competition.

    \item \textbf{SAVi}~\cite{chen2021semantic} introduces navigation to objects based on their sporadic semantic sounds, advancing beyond previous paradigms~\cite{chen2020soundspaces} that assumed constantly-sounding targets. The transformer-based architecture comprises: (1) a multimodal observation encoder that processes visual~\cite{he2016deep} and binaural audio inputs through specialized sensory pathways; (2) a goal descriptor network that dynamically predicts both relative location and object category information~\cite{mousavian2019visual}; and (3) a policy network utilizing transformer attention mechanisms~\cite{vaswani2017attention} to leverage persistent memory for long-term dependencies~\cite{parisotto2020stabilizing}. The model implements a two-stage training paradigm through decentralized distributed proximal policy optimization~\cite{wijmans2019dd} that firstly training the observation encoder without attention and subsequently freezing it while training the complete architecture with full memory capacity. The result demonstrates that effective navigation despite acoustic intermittency through cross-modal semantic associations. The approach maintains robust performance even in the presence of unheard distractor sounds~\cite{chen2020soundspaces}.
    
    \item \textbf{AVLMaps} ~\cite{huang2023audio} represents a significant advancement in embodied AI by extending traditional audio-visual navigation through the integration of natural language understanding within a comprehensive 3D spatial mapping framework. The system's architecture implements four distinct localization modules that process different perceptual modalities: a visual module employing NetVLAD~\cite{arandjelovic2016netvlad} and SuperPoint~\cite{detone2018superpoint} for feature extraction and matching; an object module utilizing open-vocabulary segmentation techniques~\cite{ghiasi2022scaling}; an area localization module for coarser spatial recognition; and an audio module that leverages audio-lingual features from pretrained models such as AudioCLIP~\cite{guzhov2022audioclip}. This multimodal approach facilitates cross-modal reasoning by converting predictions from each sensory channel into integrated voxel heatmaps through element-wise multiplication, creating a unified spatial representation that enables complex target specifications combining multiple modalities~\cite{jatavallabhula2023conceptfusion}. The results in experiments highlight the system's enhanced perceptual disambiguation capabilities through complementary modality integration, addressing a critical challenge in robotic navigation where traditional visual-only approaches often fail to disambiguate multiple instances of similar objects.
    
    \item \textbf{AVLEN}~\cite{paul2022avlen} represents a significant advancement in multimodal embodied AI systems by integrating audio-visual navigation with natural language assistance capabilities in 3D environments. It formulates the navigation task as a partially-observable Markov decision process wherein an agent localizes audio sources while strategically requesting natural language guidance when uncertainty arises. The architecture employs a hierarchical reinforcement learning framework comprising a high-level policy ($\pi_q$) that determines whether to navigate using audio-visual cues or to query an oracle, alongside two specialized lower-level policies: an audio-visual navigation policy ($\pi_g$)~\cite{chen2020soundspaces,gan2020look} and a language-based navigation policy ($\pi_{\ell}$)~\cite{anderson2018vision,fried2018speaker}. AVLEN learns when to request assistance through reinforcement learning with a carefully designed reward structure that balances navigation success against query efficiency. The model's audio processing pipeline incorporates binaural audio features, while the vision encoder employs a pre-trained ResNet18 architecture to extract visual features from RGB observations. This work establishes a foundation for more interactive embodied agents capable of effectively leveraging multimodal inputs while judiciously seeking human assistance when necessary.

    \item \textbf{CAVEN}~\cite{liu2024caven} advances embodied navigation by integrating audio-visual processing with bidirectional language interaction. Formulated as a budget-aware partially observable semi-Markov decision process~\cite{krishnamurthy2016partially}, the framework employs specialized policies for audio-visual navigation ($\pi_g$), language-based navigation ($\pi_l$)~\cite{anderson2018vision}, and question-answering ($\pi_{ques}$)~\cite{das2018embodied}, orchestrated by a selector policy ($\pi_s$) that implicitly models uncertainty. The architecture comprises: TrajectoryNet for predicting navigation paths using occupancy maps and audio goal predictions; QuestionNet for generating context-relevant questions via transformers~\cite{vaswani2017attention} and FollowerNet for providing directional guidance through cross-modal attention~\cite{tan2019lxmert}.
    
    \item \textbf{RILA}~\cite{yang2024rila} introduces a novel zero-shot semantic audio-visual navigation framework that leverages large language models (LLMs) for intelligent environmental reasoning without task-specific training. Unlike prior approaches that require extensive demonstration data, RILA implements a three-component reasoning architecture: a perception module that transforms visual and audio inputs into natural language descriptions through pre-trained vision-language models~\cite{radford2021learning,li2023blip}; an Imaginative Assistant that constructs cognitive maps by inferring room layouts and semantic relationships~\cite{gupta2017cognitive}; and a Reflective Planner that adaptively formulates navigation strategies using frontier-based exploration techniques~\cite{yamauchi1997frontier}. The system employs sophisticated audio localization by combining distance and directional estimates weighted by signal intensity~\cite{morgado2020learning}, while continuously evaluating perceptual reliability through active exploration. This architecture represents a significant advancement in cognitive navigation capabilities by integrating perceptual processing with spatial imagination and reflective planning, enabling effective navigation in complex environments without extensive training or precise perceptual information.
    
    \item \textbf{AFP}~\cite{chen2024sim2real} addresses the critical sim2real transfer challenge in audio-visual navigation by introducing a frequency-adaptive acoustic field prediction framework. Through rigorous spectral analysis, the authors systematically characterize how acoustic simulation errors vary across frequencies, revealing that lower frequencies typically exhibit larger sim2real errors due to wave effects not captured by conventional ray-tracing algorithms~\cite{savioja2015overview}. Their novel approach predicts local sound pressure fields around the agent rather than direct source localization, providing superior directional information while being more predictable from visual observations of environmental geometry~\cite{schissler2017acoustic}. This methodology builds upon theoretical foundations in computational acoustics while addressing practical robotics constraints~\cite{thrun2002probabilistic}. The hierarchical navigation framework employs a modular design that separates acoustic perception from control challenges~\cite{bansal2020combining}, utilizing a frequency-adaptive prediction strategy that intelligently selects optimal frequency bands based on both measured sim2real errors and the spectral distribution of received audio. Comprehensive validation includes both simulation-based evaluation in SoundSpaces~\cite{chen2022soundspaces} and real-world deployments using a TurtleBot platform equipped with a microphone array~\cite{nakadai2000active,valin2003robust}.
\end{itemize}
